# Supplementary material for: Sequential Strategic Screening
Source: arXiv:2301.13397 source file (2023-02-11)
Supplement: Supplementary file 1 [file sup-5_seperablecosts.tex]

\label{subsec:sepCosts}
Previous work \cite{hardt2016strategic} exhibits multiple positive results when the cost function is separable, a more well-behaved notion than when the cost is a metric. 
For reference, 
\begin{definition}
    A cost function $c(x,y)$ is called separable if it can be written as $c(x,y) = \max \{0, c_2(y) - c_1 (x)\}$, for functions $c_1, c_2 : \mathcal{X} \rightarrow \mathbb{R}$ and $c_1( \mathcal{X}) \subset c_2 (\mathcal{X})$.
\end{definition}
Our work does not focus on this type of cost functions, but a natural question is the Zig-Zag Strategy occur when the model requires that type of restricted cost function? Is there something special about the fact we use the Euclidean metric?
The answer is \emph{no} as  we show below. 
%shown in  Figure \ref{fig: seperable}.

In particular, consider the special case of linear cost functions, where cost a given $\alpha \in \mathbb{R}^d$, cost is given by 
\[  c(x,y) = \langle \alpha, (y-x) \rangle_{+} \]

Imagine a screening process with two classifiers in two dimensions with a small angle between them. In this special cost where the cost vector $\alpha$
is $[0,1]$, i.e. a vector straight upwards from the origin a Zig Zag Strategy exists. 

Observe that any point in the cone region between the two classifiers can evade the screening process by zigging right then left, with no upward movement. Since these shift vectors are orthogonal to $\alpha$, they require zero cost!

\begin{comment}
\begin{figure}[h!]
\label{fig: seperable}
\centering
\label{fig: naive}
\includegraphics[width=0.5\textwidth]{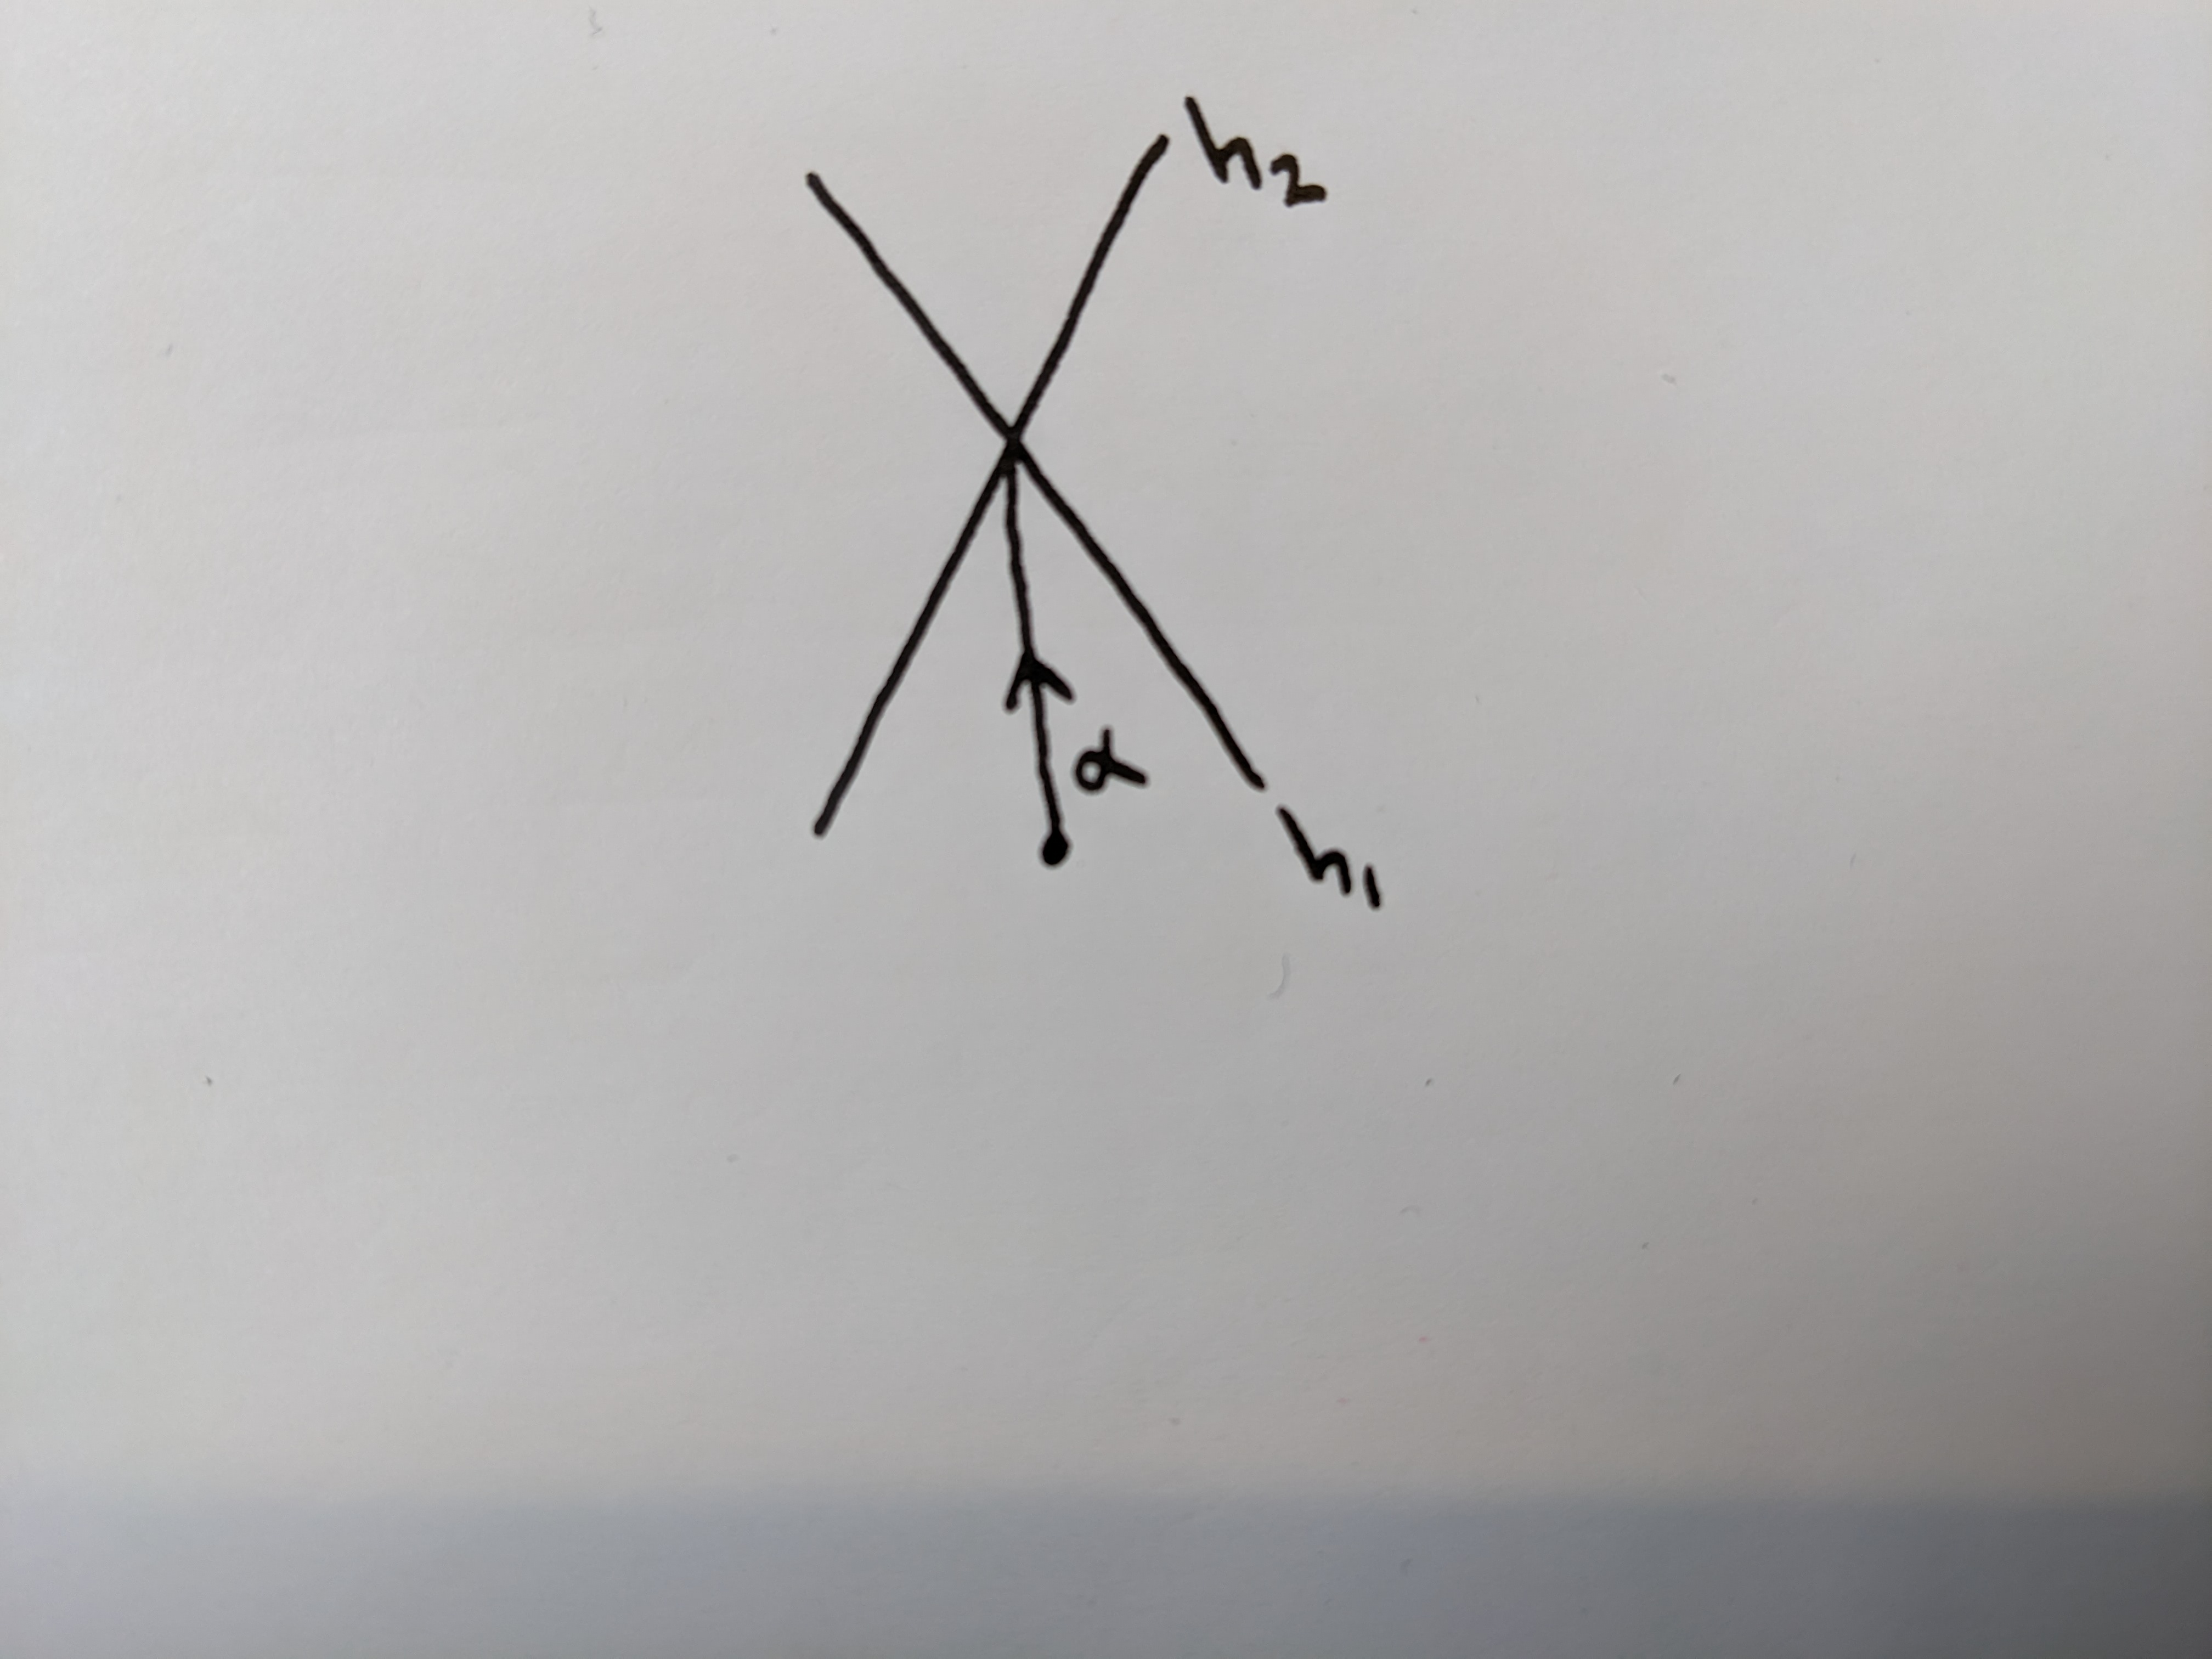}
\caption{In this case $\alpha$ is the cost vector for a linear cost function. 
Observe that any point in the cone region can evade the screenign process by zigging right then left, with no upward movement. Since these shift vectors are orthogonal to $\alpha$, they require zero cost!}
\centering
\end{figure}
This Zig-Zag Strategy can hold generically when $\alpha$ angle less than $90$ degrees  with at least one of $h_1$ or $h_2$. 
\end{comment}
