# Supplementary material for: Sequential Strategic Screening
Source: arXiv:2301.13397 source file (2023-02-11)
Supplement: Supplementary file 2 [file sup-6_hardness.tex]

\begin{proof}
\label{hardnessproof}
\juba{not formal enough yet. We need to start by setting up the problem of Bruckner or Moritz' paper (single classifier $h$) formally, then formally state the corresponding instance to our problem $(h_0,\ldots,h_0,h)$. Let's be clear what is an instance of what problem too.}
    For a given instance of strategic classification, we can reduce finding a hypothesis $h$ that attains the strategic optimum for that problem to solving for the strategic screening process.

    Consider a pipeline $\mathcal{P}=\{h_0, \dots h_0, h \} $ where the first $k-1$ classifier is the all zero linear classifier (so any point $x \in \mathcal{X}$ passes these classifiers) and the last classifier is $h$.

    Since any point $x$ passes these $k-1$ stages, they do not need to manipulate and can reserve all of their manipulation cost for the last stage. 
    Thus the best response of an actor at $x$ for evading the screening process is identical to a best response for getting the positive classification for just $h$. Thus $h$ and $\mathcal{P}$ have the same optimal strategic accuracy and an optimal defense for the classifiers in $\mathcal{P}$ is the same as just for $h$. 
    
    Given an single classifier $w$, we can thus embed it into a pipeline such that the strategic optimum and any Agent's strategy is identical and thus solving for Strategic Screening is at least as hard as strategic classification, even for linear classifiers, using the hardness result in Section 3.1 of \cite{bruckner2011stackelberg}.
    %However, observe that the assumptions for our setting are more specific than that of \cite{hardt2016strategic}, in particular we want hardness for linear classifiers and the Eucliedan Metric. 
\end{proof}

%\begin{lemma}
%The construction in \cite{hardt2016strategic} can be done in three dimensions the euclidean metric. The key feature is we need to show we can implement the metric in theorem 4.1 
%\end{lemma}

%\begin{proof}
    
%\end{proof}
